# Supplementary material for: Free Argumentative Exchanges for Explaining Image Classifiers
Source: arXiv:2502.12995 source file (2025-02-18)
Supplement: Supplementary file 1 [file appendix.tex]

\appendix

\section{Implementation}

\subsection{Player}

\subsubsection{Initialisation}

\subsubsection{Iterations}

\subsection{Training}

\subsection{Inference}

\subsection{Visualisation}
